# Supplementary material for: Animus3D: Text-driven 3D Animation via Motion Score Distillation
Source: arXiv:2512.12534 source file (2025-12-14)
Supplement: Supplementary file 1 [file 8_supp.tex]

\onecolumn
\appendix
\begin{center} \Huge \textbf{Supplementary Materials } \\
\Large \textbf{\textit{Animus3D}: Text-driven 3D Animation via Motion Score Distillation} \\
    \bigskip
\end{center}
In this supplementary material, we first compare our results with another two text-to-4D works apart from two more recent works in the main paper (Sec.~\ref{appA}).
Then in Sec~\ref{appB}, we show more results generated by our work.
Finally, in Sec.~\ref{appC}, we present more discussion including score distillation methods and selection of pretrained video diffusion models, \emph{etc}.
We strongly encourage the reader to supplementary video to better visual results.

\section{Extended Comparisons}
\label{appA}
We compare our results with two additional the-state-of-the-art text-to-4D methods, Dream-in-4D and 4d-fy~\cite{zheng2024unified, bah20244dfy}.
Quantitative results in Table~\ref{tab:app-comparison} show that our generative animation sequences  consistently surpasses the baselines in all metrics.
In Fig.~\ref{fig:app-comp} (extension of Fig.~\ref{fig:comparison} in the main paper), our results can generate substantial motion with high visual fidelity, while the two baselines could only generate 4D object with less meaningful motion (nearly static), and noticeable texture flickering.

\begin{table}[h]\centering
    \caption{\textbf{Quantitative comparison.}}
    \label{tab:app-comparison}
    \resizebox{0.5\linewidth}{!}{
    \large
    \begin{tabular}{lcccccc}
        \toprule
       Methods  & CLIP-Image$\uparrow$ & CLIP-Text $\uparrow$  & FID $\downarrow$ &  FVD $\downarrow$ \\
        \midrule

        4dfy~\cite{bah20244dfy}   & 91.85 & 42.75 & 158.9 & 863.0 \\
         Dream-in-4D~\cite{zheng2024unified}  & 91.99 & 44.30 & 204.1 & 699.3 \\
        Ours   & \textbf{93.04} & \textbf{51.05} & \textbf{88.50} & \textbf{204.1} \\
        \bottomrule
    \end{tabular}
    }
\end{table}

\section{Extended Results}
\label{appB}
Our framework can support more challenging results.
Illustrated in Fig~\ref{fig:app-res-1}, our results enables generation of more complex scenarios, such as composed 3D object and detailed text descriptions. Shown in Fig~\ref{fig:appendix-res-2}, our results can generation 4D object with diverse motion.
For example, a humanoid object can generate multiple motions like ``walking'' / ``dancing'' / ``squatting down''/ ``raising arms''.

\section{Discussions }
\label{appC}

\subsection{Relation with other score distillation methods.}
\noindent\textbf{SDI.}
Our faithful noise estimation is inspired by, but distinct from, SDI. 
The main difference lies in the temporal scheduler.
We use randomly sampled $t$ in DDIM inversion to preserve appearance (Fig.~\ref{fig:noise-faithful}). 
In contrast, SDI employs linear annealing $t$ and DDIM inversion to match the denoising trajectory, preventing over-saturation/blurriness.
Table~\ref{tab:ts} shows the annealed t slows convergence and yields worse FVD. 
% We will duly credit SDI and include more discussion to avoid overclaiming.
\begin{table}[h]\centering
    \caption{\textbf{Different time scheduler.}}
    \label{tab:ts}
    \resizebox{0.4\linewidth}{!}{
    \large
    \begin{tabular}{lccc}
        \toprule
       Time scheduler  & Linear-annealed  &  Randomly sampled (we used) \\
        \midrule
        FVD & 311.0 & 296.1  \\
        \bottomrule
    \end{tabular}
    }
\end{table}

\noindent\textbf{ProlificDreamer.}
Our method is fundamentally different from ProlificDreamer: 1) Motivation: ProlificDreamer uses LoRA to model the variational distribution of current, evolving 3D scene to be optimized, in order to address over-smoothing, over-saturation and diversity problems in SDS. In contrast, we use LoRA to model the fixed static distribution, which serves as a source distribution to provide an explicit optimization direction for motion field optimization. 2) Algorithm: we pre-train LoRA with static 3D renderings to model the static distribution then keep it frozen during optimization, unlike ProlificDreamer trains LoRA simultaneously with updated scene parameters; Also, ProlificDreamer takes the same input for both LoRA and the pretrained denoiser, our static denoiser and dynamic denoiser takes different video/text prompts. 
% 3) Our VSD comparison shows our method is much better than VSD.

\subsection{Selection of video diffusion models.}
Our MSD is robust to different T2V models, as shown in Table~\ref{tab:t2v}. Due to GPU memory limits, we selected ModelScopeT2V among these small-sized T2V models for its better motion quality.
We expect an advanced T2V model could further improve performance. 
In the motion detailization, as this module is memory-efficient, we use the advanced model Wan-T2V to obtain high-resolution, fine-grained results.

\begin{table}[h]\centering
    \caption{\textbf{Quantitative results with different T2V backbones.}}
    \label{tab:t2v}
    \resizebox{0.5\linewidth}{!}{
    \large
    \begin{tabular}{lccc}
        \toprule
       Methods  & ZeroScope & VideoCrafter2  & ModelScope (used in this paper)  \\
        \midrule
        FVD & 246.0 & 369.7 & 204.1  \\
        \bottomrule
    \end{tabular}
    }
\end{table}

\subsection{More implementation details.}
We implement our method using threestudio~\cite{threestudio2023}. 
In each iteration, we render videos with a fixed camera, where the elevation and azimuth are uniformly sampled from the range [-10, 60]$\times$[0, 360].
For the motion field, we configure the resolution and feature dimension of the Hexplanes as [100, 100, 8] and 16, respectively. The MLP head consists of a single hidden layer with a hidden dimension of 32.
In terms of motion field optimization, the learning rate for the Hexplane is set to 2e-3, while the learning rate for the MLP head is 2e-5.  
We employ several loss constraints: the MSD guidance coefficient is set to 5e-3, the ARAP loss coefficient to 12, and the TV-3D loss coefficient to 5.
For motion detailization, we use Wan2.1-1.3B~\cite{wan2025}, a rectified flow-based text-to-video model, as the base model. The image resolution is increased to 512, and the number of frames is set to $T'=25$.

\subsection{Time efficiency.}
In Table~\ref{tab:time_comparison}, we provide a comparison of optimization time. 
As mentioned in future work, a common limitation of score distillation methods is the need for several hours of optimization. 
Our method, however, converges in 5.2 hours (5,000 iterations), showing a 2$\times$ speedup over existing methods.

\begin{table}[h]\centering
    \caption{\textbf{Time expenses comparison.}}
    \label{tab:time_comparison}
    \resizebox{0.4\linewidth}{!}{
    \large
    \begin{tabular}{lcccccc}
        \toprule
       Methods   & TC4D &  AYG & AKD & Ours \\
        \midrule
        Optimization iteration ($\times$ 1000) & 17 	& 10 & 10 & \textbf{5}\\
        Average converging time (Hrs.) & 17 & 11 & 25 & \textbf{5.2}  \\
        \bottomrule
    \end{tabular}
    }
\end{table}

%%%%%%%%%%%%%%%%%
\begin{figure}[t]
    \centering
    \includegraphics[width=\linewidth]{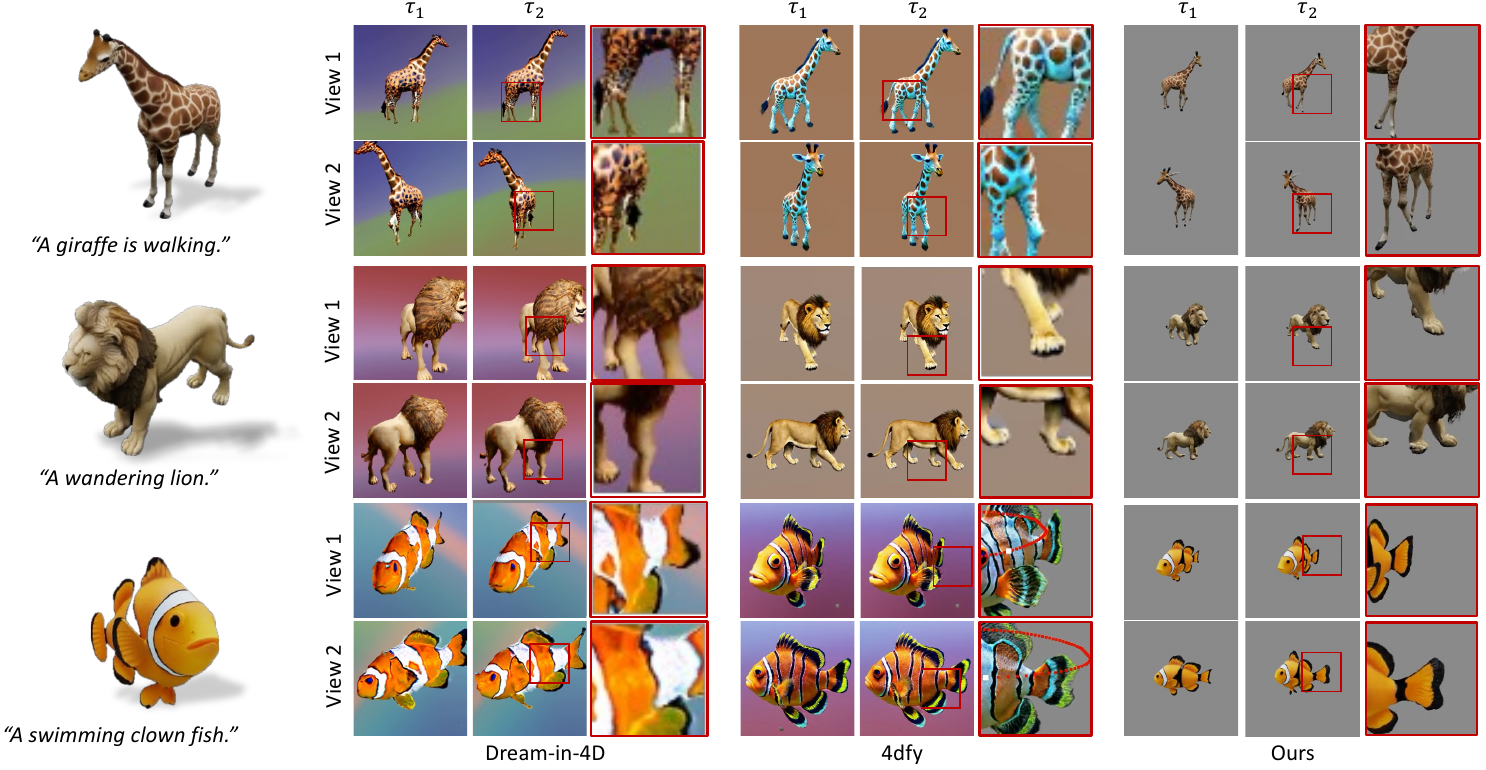}
    \caption{Comparison with two the-state-of-the-art baselines~\cite{bah20244dfy, zheng2024unified}.}
    \label{fig:app-comp}
\end{figure}

\begin{figure}[t]
    \centering
    \includegraphics[width=\linewidth]{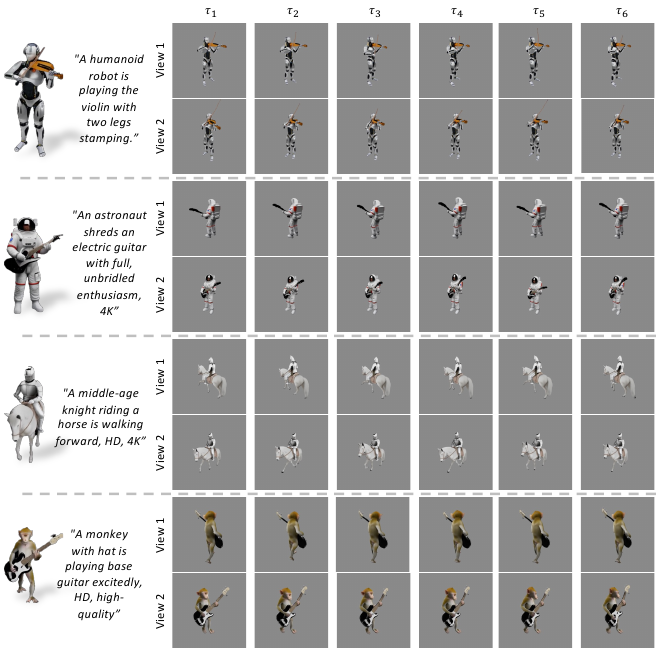}
    \caption{Our framework enables generation of more complex 3D animations, \emph{e.g.} composed 3D object, and detailed text description.}
    \label{fig:app-res-1}
\end{figure}

\begin{figure}[t]
    \centering
    \includegraphics[width=\linewidth]{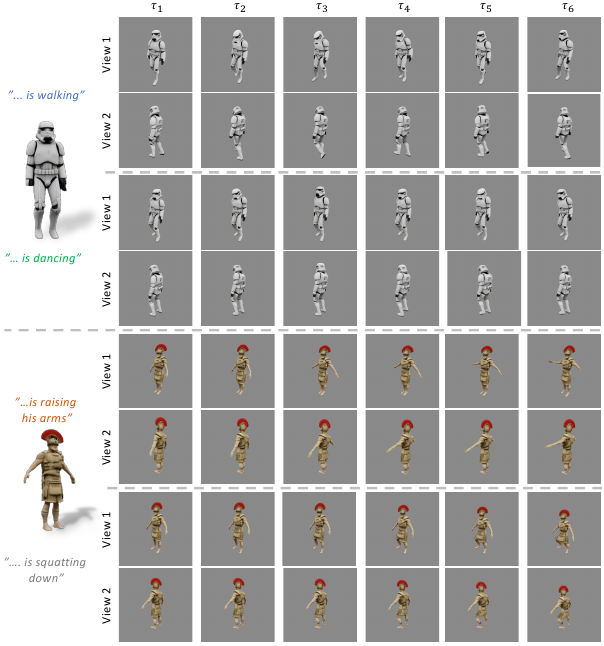}
    \caption{Our framework can generate different 3D animation with diverse text prompts given arbitrary static 3D object.}
    \label{fig:appendix-res-2}
\end{figure}
